# Supplementary material for: Decentralized Entropic Optimal Transport for Distributed Distribution Comparison
Source: arXiv:2301.12065 source file (2024-07-22)
Supplement: Supplementary file 1 [file appendix.tex]

\newpage
\appendix
\onecolumn
\section{Delayed Proofs}\label{app:proof}

The precision of the proposed approximation is guaranteed under mild assumptions:
\begin{itemize}
    \item \textbf{Assumption 1.} The kernel in the objective is a GIP kernel, i.e., $\kappa(x,y)=g(\phi(x,y),\|x\|,\|y\|)$ and $g$ is a $G$-Lipschitz continuous function with respect to $\phi$.
    \item \textbf{Assumption 2.} Both the kernel $\kappa$ and its approximation $\hat{\kappa}$ are bounded, i.e., $|\kappa(x,y)|\leq b$ and $|\hat{\kappa}(x,y)|\leq b$ for some $b\geq 1$.
\end{itemize}
\begin{theorem}\label{thm:kernel-approx}
Let $K\in\mathbb{R}^{N\times M}$ be the matrix defined by the GIP kernel in~\eqref{eq:GIP} and $\widehat{K}$ be the approximation achieved via~\eqref{eq:Kmat}.
Based on the assumptions 1-2, with probability at least $1-\delta$, we have $\|K-\widehat{K}\|\leq G(N+M)\Bigl( \sqrt{\frac{32\pi^2}{P}\log\frac{2(N+M)}{\delta}} + \frac{8\pi}{3P}\log\frac{2(N+M)}{\delta} \Bigr)$.
\end{theorem}
Theorem~\ref{thm:kernel-approx} means that $\widehat{K}\rightarrow K$ when $P\rightarrow\infty$. 
$P = \mathcal{O}(\epsilon^{-2})$ achieves an approximation error $\epsilon>0$. 
Theorem~\ref{thm:kernel-approx} is based on the Lemma 4.1 in~\cite{khanduri2021decentralized}.
More details can be found at Appendix~\ref{app:proof}.

\subsection{The proof of Theorem~\ref{thm:approx_error}}

\begin{proof}
Let $u_1,v_1=\arg\sup_{u, v \in \mathcal{C}(\mathcal{X})} \mathbb{E}_{(i, j)\sim E}[\mathbb{E}_{x\sim \mu_i,y\sim\gamma_j}[f_{\varepsilon}(x,y,u,v)]]$ be the optimal dual functions of $W_{\varepsilon}(\mu, \gamma)$.
Similarly, let $u_2,v_2$ be the optimal dual functions of $\widetilde{W}_{\varepsilon}(\mu, \gamma)$.
We have
\begin{eqnarray*}
\begin{aligned}
    |\widetilde{W}_{\varepsilon}(\mu, \gamma)-W_{\varepsilon}(\mu, \gamma)|
    &\leq
    \begin{cases}
        \sum_{i,j}(e_{ij}-p_i q_j)\mathbb{E}_{x\sim \mu_i,y\sim\gamma_j}[f_{\varepsilon}(x,y,u_1,v_1)] &\text{if}~\widetilde{W}_{\varepsilon}(\mu, \gamma)\geq W_{\varepsilon}(\mu, \gamma)\\
        \sum_{i,j}(p_i q_j - e_{ij})\mathbb{E}_{x\sim \mu_i,y\sim\gamma_j}[f_{\varepsilon}(x,y,u_2,v_2)] &\text{if}~\widetilde{W}_{\varepsilon}(\mu, \gamma)< W_{\varepsilon}(\mu, \gamma)\\
    \end{cases}\\
    &\leq 
    \sideset{}{_{i,j}}\sum|e_{ij}-p_i q_j|\sideset{}{_{u\in\{u_1,u_2\},v\in\{v_1,v_2\}}}\max\mathbb{E}_{x\sim \mu_i,y\sim\gamma_j}[f_{\varepsilon}(x,y,u,v)]\\
    &\leq
    \sideset{}{_{i,j}}\sum|e_{ij}-p_i q_j|\sideset{}{_{u,v\in\mathcal{C}_{\mathcal{X}}}}\sup\mathbb{E}_{x\sim \mu_i,y\sim\gamma_j}[f_{\varepsilon}(x,y,u,v)]\\
    &=
    \sideset{}{_{i,j}}\sum|e_{ij}-p_i q_j|W_{\varepsilon}(\mu_i, \gamma_j)\\
    &\leq \sideset{}{_{i,j}}\max W_{\varepsilon}(\mu_i, \gamma_j)\sideset{}{_{i,j}}\sum|e_{ij}-p_i q_j|\\
    &\leq \tau\sigma.
    % &\leq \max_{i,j}W_{\varepsilon}(\mu_i, \gamma_j)\Bigl(\sum_{i,j}t_{ij}+ \sum_{i,j}p_i q_j\Bigr)\\
    % &= 2\tau.
\end{aligned}
\end{eqnarray*}
\end{proof}

\subsection{The proof of Theorem~\ref{thm:kernel-approx}}

% \begin{theorem}\label{thm:kernel-approx}
% Let $K\in\mathbb{R}^{N\times M}$ be the matrix defined by the GIP kernel in~\eqref{eq:GIP} and $\widehat{K}$ be the approximation achieved via~\eqref{eq:Kmat}.
% Based on the assumptions 1-2, with probability at least $1-\delta$, we have $\|K-\widehat{K}\|\leq G(N+M)\Bigl( \sqrt{\frac{32\pi^2}{P}\log\frac{2(N+M)}{\delta}} + \frac{8\pi}{3P}\log\frac{2(N+M)}{\delta} \Bigr)$.
% \end{theorem}

\begin{proof}
The proof of this Theorem~\ref{thm:kernel-approx} is based on the Lemma 4.1 in~\cite{khanduri2021decentralized}.
We aims to approximately calculate a $N\times M$ kernel matrix $K$, which can be considered as a sub-block matrix of the $(N+M)\times (N+M)$ full kernel matrix base on given $N+M$ data samples.
This full kernel matrix can be denoted as $K_{full}\in {\mathbb{R}}^{(N+M)\times (N+M)}$.
The employed privacy-preserving Kernel Approximation algorithm, i.e., {\bf{Algorithm 1}}, can be considered as a partial version of the Algorithm 1 in~\cite{khanduri2021decentralized}.
As a result, we can utilize the theoretical result, i.e., Lemma 4.1 in~\cite{khanduri2021decentralized} to estimate the approximate level of $\widehat{K}_{full} \in {\mathbb{R}}^{(N+M)\times (N+M)}$ obtained through the Algorithm 1 in~\cite{khanduri2021decentralized}.
Based on the assumptions 1-2, with probability at least $1-\delta$, we have
$$\|K_{full} - \widehat{K}_{full}\|\leq G(N+M)\Bigl( \sqrt{\frac{32\pi^2}{P}\log\frac{2(N+M)}{\delta}} + \frac{8\pi}{3P}\log\frac{2(N+M)}{\delta} \Bigr).$$
For the reason that $K$ is a sub-block matrix of $K_{full}$, so as the approximated $\widehat{K}$ with respect to $\widehat{K}_{full}$,
Furthermore, based on the assumptions 1-2, with probability at least $1-\delta$, we have
$$
\|K - \widehat{K}\|\le \|K_{full} - \widehat{K}_{full}\|\leq G(N+M)\Bigl( \sqrt{\frac{32\pi^2}{P}\log\frac{2(N+M)}{\delta}} + \frac{8\pi}{3P}\log\frac{2(N+M)}{\delta} \Bigr),
$$which indicates the result of this Theorem.
\end{proof}

\subsection{The proof of Theorem~\ref{thm:error-bound}}

\begin{proof}
Let $\hat{u}^*,\hat{u}^*=\arg\max_{u,v}F_{\varepsilon}(u,v;\widehat{K},E)$ be the optimal solution of the problem~\eqref{eq:sample-eot} given approximated kernel $\widehat{K}$, and $\tilde{u}^*,\tilde{u}^*=\arg\max_{u,v}F_{\varepsilon}(u,v;K,E)$ be the optimal solution of the problem~\eqref{eq:sample-eot} given real kernel $K$.
In order to prove \eqref{eq:expect-error-bound}, we first establish the connections with the algorithmic convergence error, the approximated kernel error and the mismatch between the storage and communication protocols.
In particular, applying the triangle inequality, we have
\begin{eqnarray*}
\begin{aligned}
&\mathbb{E}\left[\big|F_{\varepsilon}(\hat{u}^{t}, \hat{v}^{t};\widehat{K},E)-W_{\varepsilon}(\mu,\gamma) \big| \right]  \\
\leq&\mathbb{E} \left[ \big| F_{\varepsilon}(\hat{u}^{t}, \hat{v}^{t};\widehat{K},E) - F_{\varepsilon}(\hat{u}^{*}, \hat{v}^{*};\widehat{K},E) \big|\right] + \big| F_{\varepsilon}(\hat{u}^{*}, \hat{v}^{*};\widehat{K},E) - F_{\varepsilon}(\tilde{u}^{*}, \tilde{v}^{*};K,E) \big| \\
&+ \big| F_{\varepsilon}(\tilde{u}^{*}, \tilde{v}^{*};K,E) - W_{\varepsilon}(\mu,\gamma) \big| \\
=&\mathbb{E} \big[ \underbrace{\big| F_{\varepsilon}(\hat{u}^{t}, \hat{v}^{t};\widehat{K},E) - F_{\varepsilon}(\hat{u}^{*}, \hat{v}^{*};\widehat{K},E) \big|}_{\hbox{convergence error by Lemma~\ref{le:algorithm-error}}}\big] + \underbrace{\big| F_{\varepsilon}(\hat{u}^{*}, \hat{v}^{*};\widehat{K},E) - F_{\varepsilon}(\tilde{u}^{*}, \tilde{v}^{*};K,E) \big|}_{\hbox{approximated kernel error}} \\
&+ \underbrace{\big| \widetilde{W}_{\varepsilon}(\mu,\gamma) - W_{\varepsilon}(\mu,\gamma) \big|}_{\hbox{gap by Theorem~\ref{thm:approx_error}}}.
\end{aligned}
\end{eqnarray*}
The first and third terms in the above equation have been analyzed in Lemma~\ref{le:algorithm-error} and Theorem~\ref{thm:approx_error} respectively.
The key issue is to analyze the approximated kernel error term.

%\subsection{The proof of kernel approximation error estimation \eqref{eq:kernel-error}}\label{appendix:kernel error}

%\begin{proof}
Each $f_{\varepsilon} (x,y,u,v)$ is typically convex and Lipschitz continuous with respect to $(u, v)$~\cite{genevay2016stochastic}.
The objective function $F_{\varepsilon}$ is Lipschitz continuous with respect to $(u,v)$.
Further based on the definition of $f_{\varepsilon}^{(i,j)}$, it is obvious that $f_{\varepsilon}^{(i,j)}$ is a liner function with respect to $\kappa (x_n^{(i)},y_m^{(j)})$.
On the whole, the objective function $F_{\varepsilon}$ can be considered as a linear function with respect to kernel matrix $K$ and thus also is Lipschitz continuous with respect to $K$.
According to \cite{dempe2015lipschitz}[Lemma 3.1], if we model $K$ as the varible of the parametric optimization problem
$$
\phi(K) = \max_{u,v} F_{\varepsilon} \big( u, v; K, E \big).
$$We can conclude that the optimal value function $\phi\big(K\big)$ with respect to $K$ is $L_{\kappa}$-Lipschitz continuous, i.e.,
$$
\big| F_{\varepsilon}(\hat{u}^{*}, \hat{v}^{*};\widehat{K},E) - F_{\varepsilon}(\tilde{u}^{*}, \tilde{v}^{*};K,E)  \big| = \big| \phi(\widehat{K}) - \phi(K) \big|\le L_{\kappa} \big\| \widehat{K} - K \big\|.
$$
%According to Assumption 4, it can be obtained that $L_{\kappa}$ can be denoted as $\frac{\hat{L}_{\kappa} I^2}{N^2}$ with $\hat{L}_{\kappa}$ be the modified constant.

As a consequence of Theorem~\ref{thm:approx_error}, Theorem~\ref{thm:kernel-approx}, and Lemma~\ref{le:algorithm-error}, we have that for the problem in~\eqref{eq:sample-eot} with the kernel $\widehat{K}$ derived by Algorithm~\ref{Algo-Kernel}, let $\left\{\left(u^t,v^t\right)\right\}$ be the sequence generated by Algorithm~\ref{Algo-MRBCD}. 
Define $\hat{u}^{t} = \frac{1}{t}\sum_{\ell=1}^{t} u^{\ell}$, and $\hat{v}^{t} = \frac{1}{t} \sum_{\ell=1}^{t} v^{\ell}$.
Based on the assumptions 1-3, with probability at least $1-\delta$, we have 
\begin{eqnarray}\label{eq:expect-error-bound2}
\begin{aligned}
&\mathbb{E}|F_{\varepsilon}(\hat{u}^{t}, \hat{v}^{t};\widehat{K},E)-W_{\varepsilon}(\mu,\gamma)| \\
\leq& \mathcal{O}\Bigl(\frac{IJ\left( (\sqrt{t} + L_{F_{\varepsilon}})R_0^2 + \sqrt{t}R^2\right)}{t}\Bigr) + L_{\kappa}G(N+M)\Bigl( \sqrt{\frac{32\pi^2}{P}\log\frac{2(N+M)}{\delta}} + \frac{8\pi}{3P}\log\frac{2(N+M)}{\delta} \Bigr) \\
&+ \tau\sigma \\
\leq& \mathcal{O}\Bigl(\frac{IJ}{\sqrt{t}} + (N+M)\sqrt{\frac{1}{P}\log\frac{2(N+M)}{\delta}}+\sigma \Bigr). 
\end{aligned}
\end{eqnarray}
To emphasis, the second term in~\eqref{eq:expect-error-bound2} has close relationship with the number of samples per agent (i.e., $N_i$ and $M_j$).
We propose a worst case analysis, while it can be modified properly with well-designed $N_i$ and $M_j$.

% where $L_{\kappa}$ is the Lipschitz constant of the optimal dual objective with the kernel as a parameter, $R_0=\min_{u,v\in \mathcal{C}^*}\|(u^0,v^0)-(u,v)\|_2$, and $\mathcal{C}^*$ is the optimal solution set of~\eqref{eq:sample-eot}.
% \begin{eqnarray}\label{eq:expect-error-bound}
% \begin{aligned}
%     &\mathbb{E}|F_{\varepsilon}(\hat{u}^{t}, \hat{v}^{t};\widehat{K},E)-W_{\varepsilon}(\mu,\gamma)|
%     \leq \mathcal{O}\Biggl(\tau\sigma +\\
%     &\frac{(\sqrt{t} + L)R_0^2 + \sqrt{t}R^2}{t} + L_{\kappa}GN\Bigl(\sqrt{\frac{32\pi^2}{P}\log\frac{2N}{\delta}}\Bigr)\Biggr),
% \end{aligned}
% \end{eqnarray}
% where $L_{\kappa}$ is the Lipschitz constant of the optimal dual objective with the kernel $K$ as a parameter, and the remaining notations are defined in Theorem~\ref{thm:approx_error}, Theorem~\ref{thm:kernel-approx}, and Lemma~\ref{le:algorithm-error}.
\end{proof}

\begin{figure}
    \centering
    \subfigure[$W_{\varepsilon}(\mathcal{N}_1,\mathcal{N}_2)$, $L=1$]{
    \includegraphics[height=5.1cm]{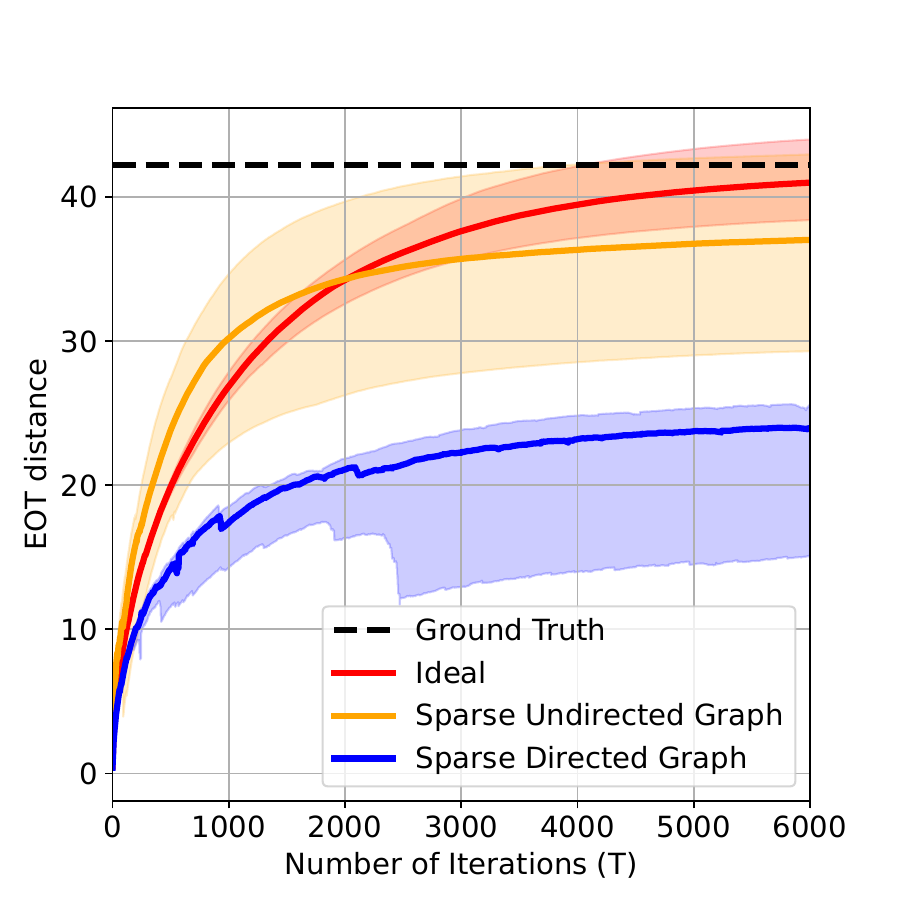}
    }
    \subfigure[$W_{\varepsilon}(\mathcal{N}_1,\mathcal{N}_2)$, $L=4$]{
    \includegraphics[height=5.1cm]{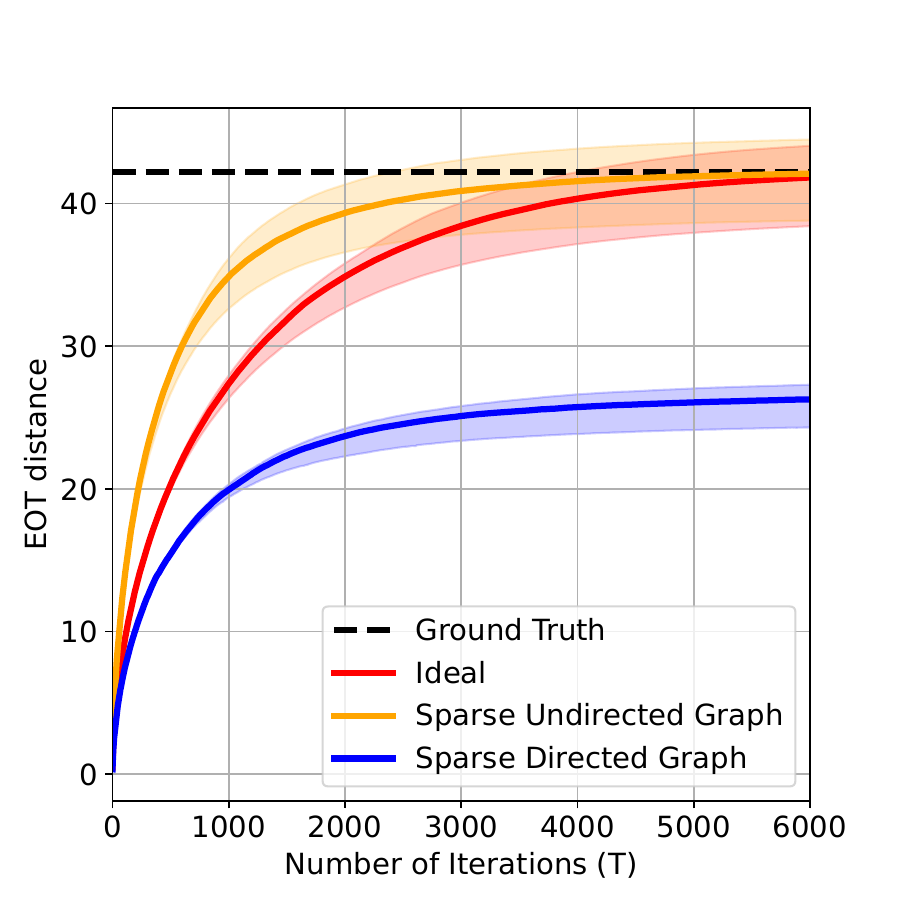}
    }
    \subfigure[$W_{\varepsilon}(\mathcal{N}_1,\mathcal{N}_2)$, $L=8$]{
    \includegraphics[height=5.1cm]{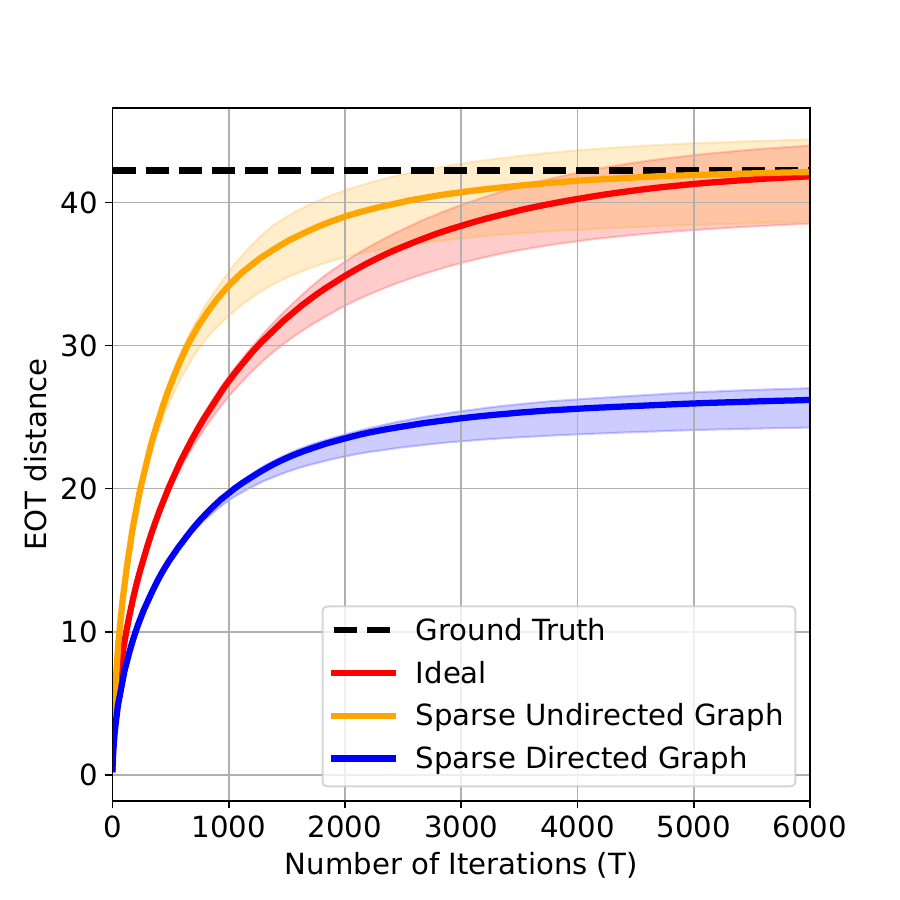}
    }
    \subfigure[$W_{\varepsilon}(\mathcal{M}_1,\mathcal{M}_2)$, $L=1$ (i.i.d.)]{
    \includegraphics[height=5.1cm]{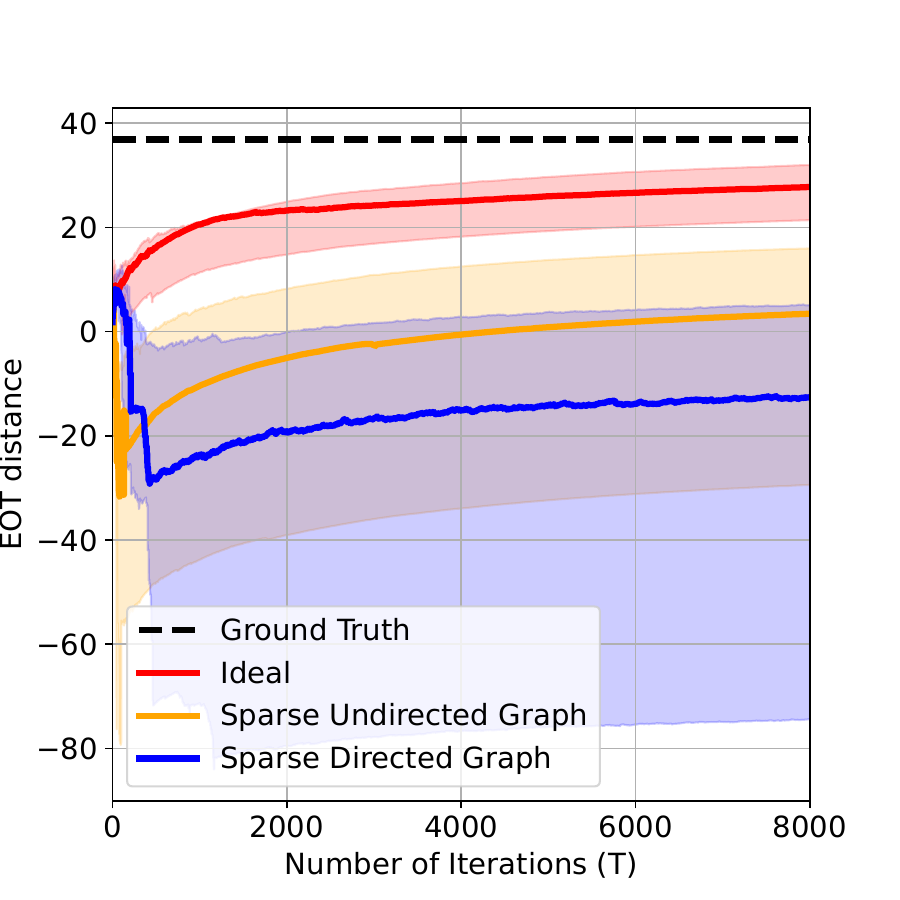}
    }
    \subfigure[$W_{\varepsilon}(\mathcal{M}_1,\mathcal{M}_2)$, $L=4$ (i.i.d.)]{
    \includegraphics[height=5.1cm]{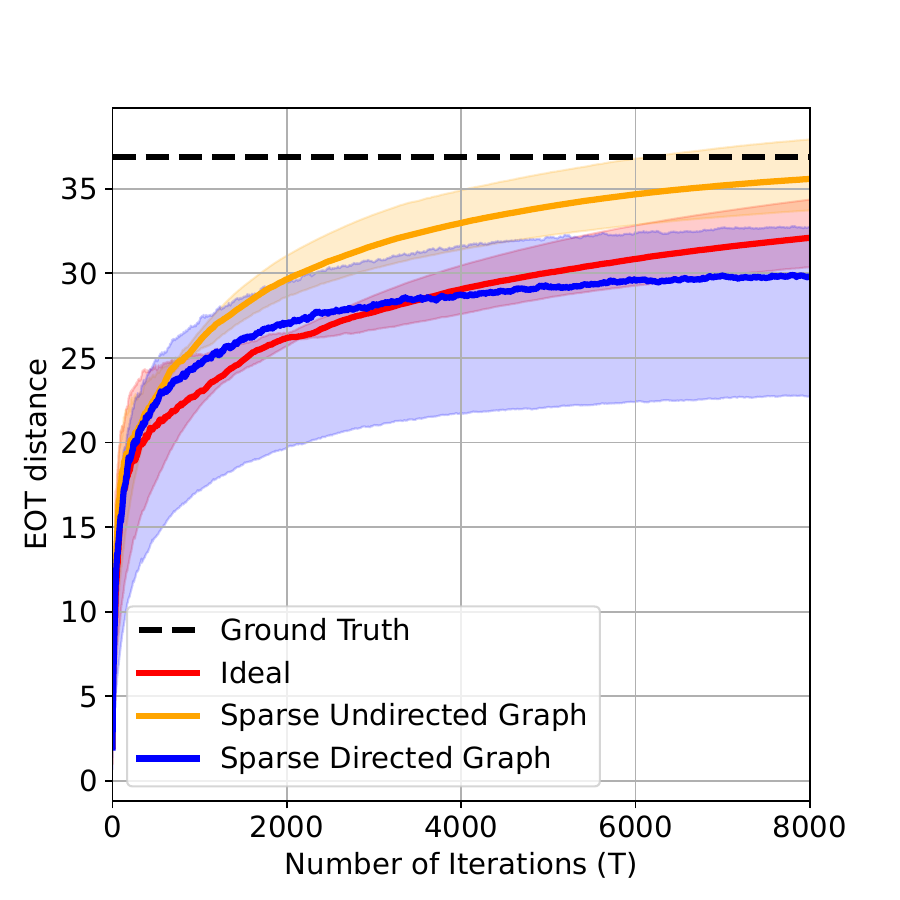}
    }
    \subfigure[$W_{\varepsilon}(\mathcal{M}_1,\mathcal{M}_2)$, $L=8$ (i.i.d.)]{
    \includegraphics[height=5.1cm]{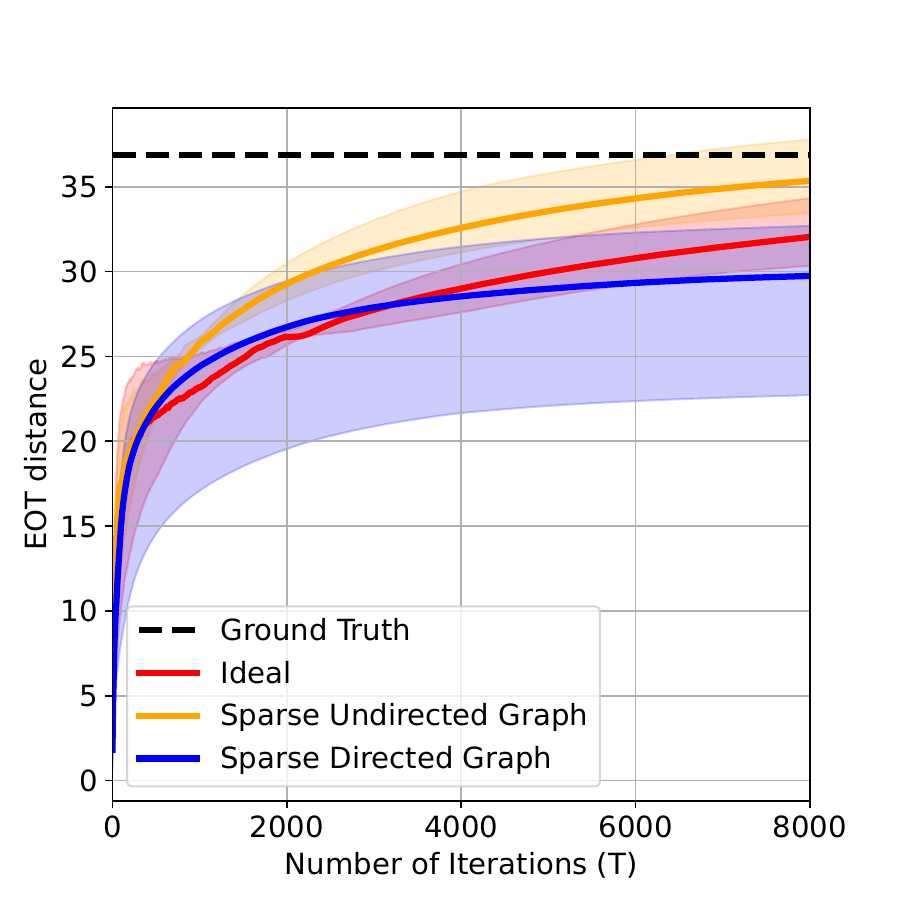}
    }
    \subfigure[$W_{\varepsilon}(\mathcal{M}_1,\mathcal{M}_2)$, $L=1$ (non-i.i.d.)]{
    \includegraphics[height=5.1cm]{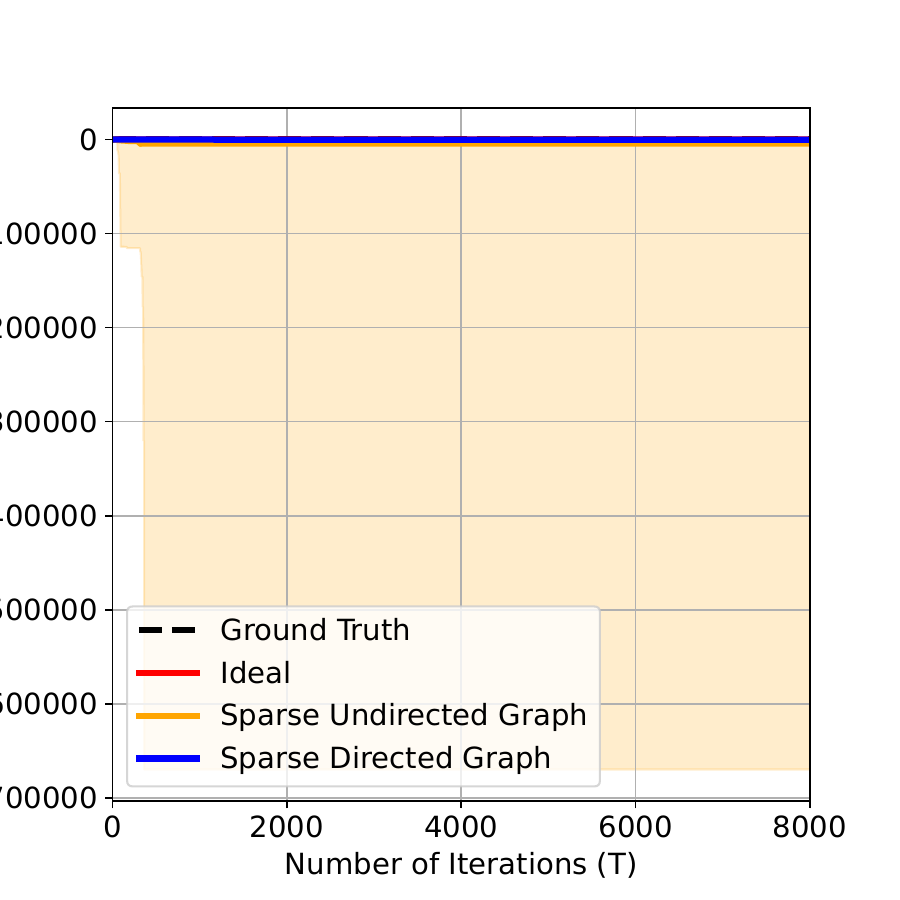}
    }
    \subfigure[$W_{\varepsilon}(\mathcal{M}_1,\mathcal{M}_2)$, $L=4$ (non-i.i.d.)]{
    \includegraphics[height=5.1cm]{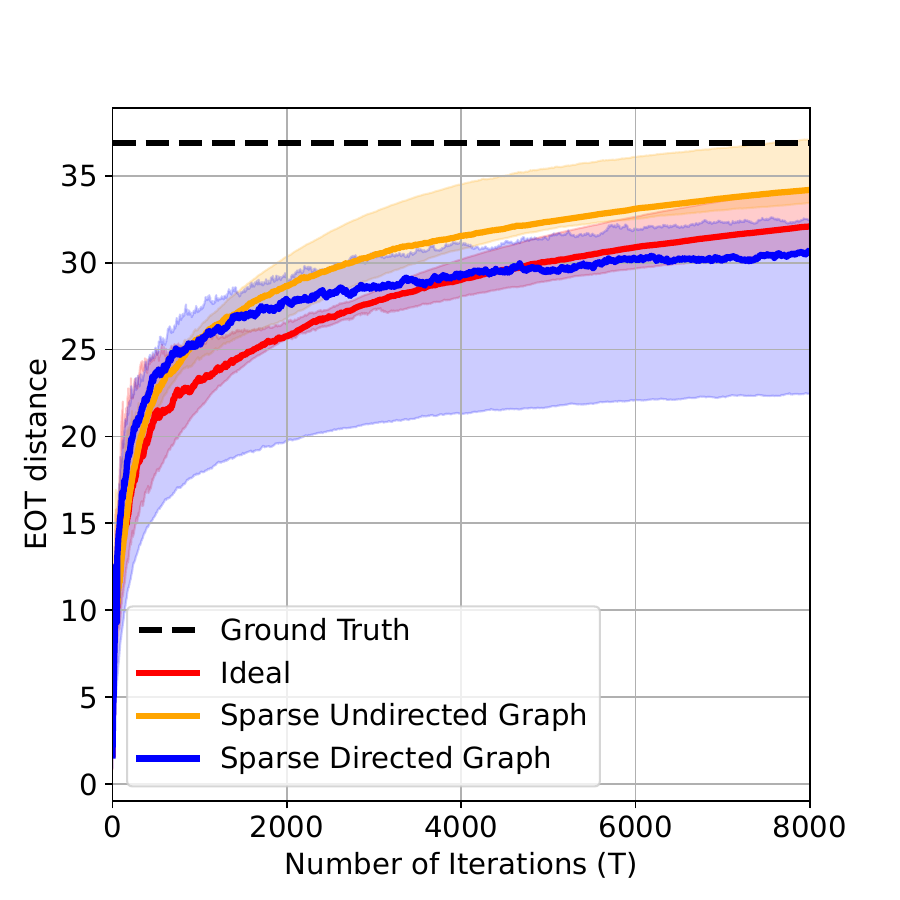}
    }
    \subfigure[$W_{\varepsilon}(\mathcal{M}_1,\mathcal{M}_2)$, $L=8$ (non-i.i.d.)]{
    \includegraphics[height=5.1cm]{figures/eot_protocols/w_gmm_niid_protocol_L8.pdf}
    }
    \caption{The computation of $W_{\varepsilon}(\mathcal{N}_1,\mathcal{N}_2)$. 
    In this experiments, we consider two domains, each of which contains eight agents respectively. In each domain, the samples of Gaussian distributions are randomly scattered to the agents, and each agent contains $50$ samples. 
    In each subfigure, the block dotted line indicates the $W_{\varepsilon}(\mathcal{N}_1,\mathcal{N}_2)$ computed by the classic Sinkhorn-scaling algorithm. The red, orange, and blue curves indicates the average convergence curves of our MRBCD algorithm when applying binary data, and the communication protocols they used are identical to the storage protocol (ideal), random probabilities defined on a sparse undirected bipartite graph, and random probabilities defined on a sparse directed bipartite graph, respectively.}
    \label{fig:eot_protocol}
\end{figure}

\begin{figure}[t]
\centering
\subfigure[$W_{\varepsilon}(\mathcal{N}_1,\mathcal{N}_2)$]
{
        \includegraphics[height=5.6cm]{figures/g_exp_I.pdf}
}
\subfigure[$W_{\varepsilon}(GMM_1,GMM_2)$]
{
        \includegraphics[height=5.6cm]{figures/gm_exp_I.pdf}
}
\caption{The influence of the number of servers in each domain.}\label{fig:syn_exp_I}
\end{figure}

\begin{figure}[t]
\centering
\subfigure[$L=2$]{
        \includegraphics[height=4.8cm]{figures/g_exp_topo_L2.pdf}
}
\subfigure[$L=5$]{
        \includegraphics[height=4.8cm]{figures/g_exp_topo_L5.pdf}
}
\subfigure[$L=5$]{
        \includegraphics[height=4.8cm]{figures/gm_exp_topo_L5.pdf}
}
\caption{(a, b) The robustness of our method to the communication protocol when computing $W_{\varepsilon}(\mathcal{N}_1,\mathcal{N}_2)$.
(c) The influence of communication protocol when computing $W_{\varepsilon}(GMM_1,GMM_2)$. In this experiment, we set $L=5$ and $P=1000$.}\label{fig:syn_exp_comm}
\end{figure}

\section{Implementation Details and More Experimental Results}\label{app:exp}
\subsection{Synthetic experiments}
In order to gain insight into the effect of the number of servers on the algorithm, we set $I,J\in\{5, 10, 20\}$, $L=\text{round}(0.7I)$, and the number of samples to be $N=M=2000$. 
From the experimental results showed in Figure~\ref{fig:syn_exp_I}, we can find that as the number of servers increases, convergence is faster at the beginning of the iteration and is accompanied by a more pronounced oscillation.

Additionally, Figure~\ref{fig:syn_exp_comm} shows more experimental results, visualizing the impacts of different communication protocols.

\subsection{Real-world experiments}
\begin{table}[tb!]
\centering
\caption{Summary of the domains used in the experiments}\label{tab:sum}
\begin{small}
\begin{tabular}{@{}c|c|c|c|c|c@{}}
\hline\hline
Problem   
& Domains   
& Datasets 
& \#Samples
& \#Features 
& Abbr.\\
\hline

Digits & USPS           & USPS   & $1,800$ & $256$  & U\\

  & MNIST      & MNIST   & $2,000$  & $256$  & M\\
 \hline
 Objects & Art & Office-home & $2,427$ & $2,048$ & Ar \\
& Clipart & Office-home & $4,365$ & $2,048$ & Cl \\
& Product & Office-home & $4,439$ & $2,048$ & Pr \\
& Real-World & Office-home & $4,357$ & $2,048$ & Rw \\
\hline\hline
\end{tabular}
\end{small}
\end{table}

\begin{table}[tb!]
\centering
\caption{Comparisons on classification accuracy in distributed domain adaptation tasks}\label{tab:officehome}
\begin{small}
\begin{tabular}{@{}c|c|ccc|cc@{}}
\hline\hline
\multirow{2}{*}{Domains}     
% & \multirow{2}{*}{Method}   
& Source only
& 
&Centralized
&
&
\multicolumn{2}{c}{Decentralized (Ours)} \\ 

& 1NN
& EMD
& Sinkhorn
& OT-LpL1

& MRBCD$_K$
& MRBCD$_{\widehat{K}}$\\
\hline

Ar$\rightarrow$Cl    & $0.433$   & $0.471$  & $0.492$  & $0.490$ & $0.483$ & $0.458$\\ 
Ar$\rightarrow$Pr    & $0.594$   & $0.642$  & $0.673$  & $0.633$ & $0.665$ & $0.639$\\
Ar$\rightarrow$Rw    & $0.667$   & $0.677$  & $0.721$  & $0.686$ & $0.738$ & $0.705$\\
\hline
Cl$\rightarrow$Ar   & $0.445$   & $0.504$  & $0.509$  & $0.478$ & $0.531$ & $0.509$\\
Cl$\rightarrow$Pr    & $0.536$   & $0.647$  & $0.617$  & $0.642$ & $0.632$ & $0.606$\\
Cl$\rightarrow$Rw    & $0.589$   & $0.638$  & $0.657$  & $0.664$ & $0.654$ & $0.618$\\
\hline
Pr$\rightarrow$Ar    & $0.488$   & $0.516$  & $0.532$  & $0.494$ & $0.538$ & $0.506$\\
Pr$\rightarrow$Cl    & $0.414$   & $0.455$  & $0.465$  & $0.450$ & $0.469$ & $0.425$\\
Pr$\rightarrow$Rw    & $0.683$   & $0.707$  & $0.725$  & $0.714$ & $0.735$ & $0.704$\\
\hline
Rw$\rightarrow$Ar    & $0.592$   & $0.611$  & $0.622$  & $0.605$ & $0.621$ & $0.598$\\
Rw$\rightarrow$Cl    & $0.450$   & $0.498$  & $0.505$  & $0.509$ & $0.494$ & $0.463$\\
Rw$\rightarrow$Pr    & $0.729$   & $0.749$  & $0.778$  & $0.770$ & $0.773$ & $0.736$\\

\hline\hline
\end{tabular}
\end{small}
\end{table}
The distributed domain adaptation task is dedicated to solving the domain adaptation problem in the case where both source and target domain data are scattered over different agents. The aim is to use the label information available in the source domain $\mathcal{X}$ to learn a classifier $f^*$ that can be applied on the target domain $\mathcal{Y}$ without label information.
Specifically, suppose we have the source domain data $X_{i}=\{x_{n}^{(i)}\}_{n=1}^{N_i}$ associated with the class labels, and the target domain data $Y_{j}=\{y_{m}^{(j)}\}_{m=1}^{M_j}$ with unknown labels.
Based on our algorithm MRBCD, each target agent $j$ can obtain an optimal coupling $\{\Pi_{ij}\}_{i=1}^{I}$. 
Then, according to~\cite{courty2017joint}, when the probability measures $\mu$ and $\gamma$ are uniform, we can derive the barycentric mapping as $\widehat{X}=N \Pi Y$, where $\Pi=[\Pi_{ij}]$ is the complete coupling and $\widehat{X}$ is the transported data of the source domain. 
Eventually, we can train the 1NN classifier $f$ given the transported data $\widehat{X}$ and perform classification prediction on the target domain data.

We further conduct experiments on the object recognition task. 
Here, we use the Office-home dataset~\cite{2017Deep}.
A summary of the properties of each domain used in this paper is provided in Table\ref{tab:sum}.
The Office-home dataset contains around 15500 images coming from four different domains: Art (artistic images in the form of sketches, paintings, etc), Clipart (collection of clipart images), Product (images of objects without a background) and RealWorld (images of objects captured with a regular camera). 
For this problem, all the experiments are based on pre-trained ResNet-50~\cite{DBLP:journals/corr/HeZRS15}. We consider 12 transfer tasks for the Art (\textbf{Ar}), Clipart (\textbf{Cl}), Product (\textbf{Pr}) and Real-World (\textbf{Rw}) domains for all combinations of source and target for the 4 domains. The results are shown in the Table\ref{tab:officehome}.

\textbf{Hyperparameter setting.}
As for the experimental setup, we scattered the source and target domain data over four agents and set $L=7$ and $P=10000$.
For all the EOT-based method, we apply grid search, finding the optimal weight of regularizer $\varepsilon\in \{2, 1, 0.5, 0.1, 0.05\}$.
For our method, the learning rate is set in $\{1, 0.5, 0.1, 0.01, 0.001\}$.
